# Supplementary material for: Effect of strain and many-body corrections on the band inversions and topology of bismuth
Source: arXiv:2102.02018 source file (2022-08-25)
Supplement: Supplementary file 1 [file supplemental-bands.pdf]

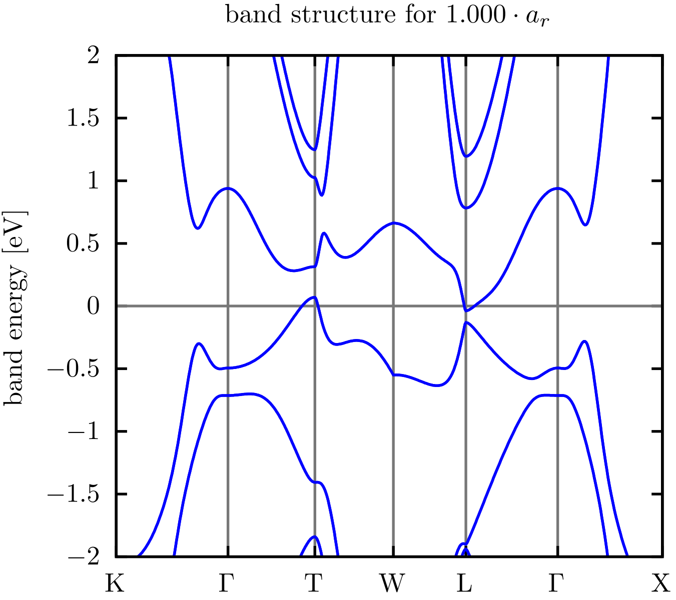

band structure for $1.000 \cdot a_r$
band energy [eV]
2
1.5
1
0.5
0
−0.5
−1
−1.5
−2
K
Γ
T
W
L
Γ
X

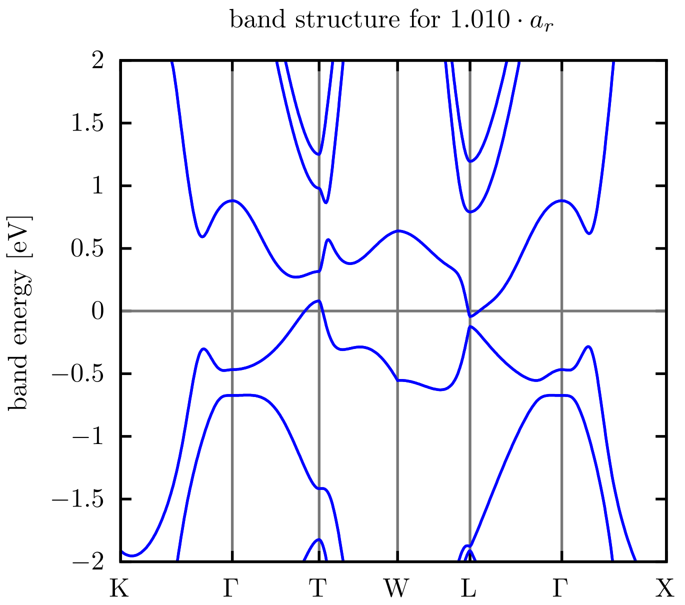
band structure for $1.010 \cdot a_r$
band energy [eV]
2
1.5
1
0.5
0
−0.5
−1
−1.5
−2
K
Γ
T
W
L
Γ
X

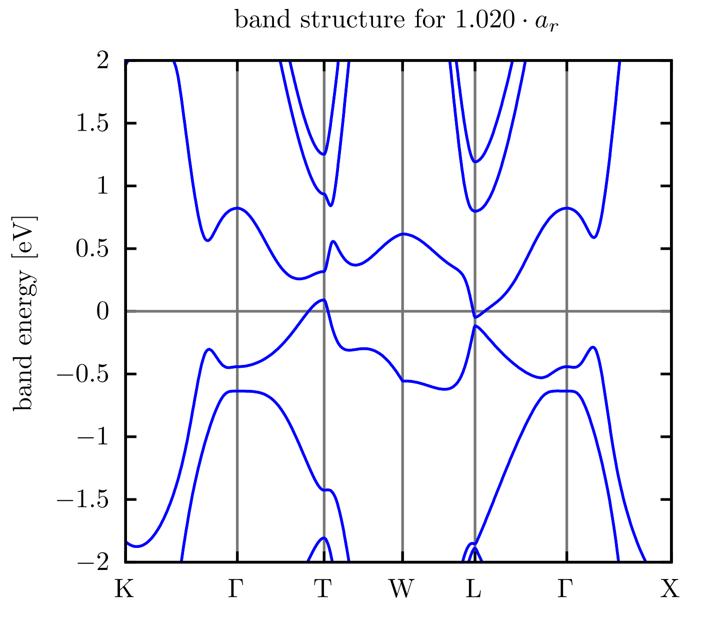

band structure for $1.020 \cdot a_r$
band energy [eV]
2
1.5
1
0.5
0
−0.5
−1
−1.5
−2
K
Γ
T
W
L
Γ
X

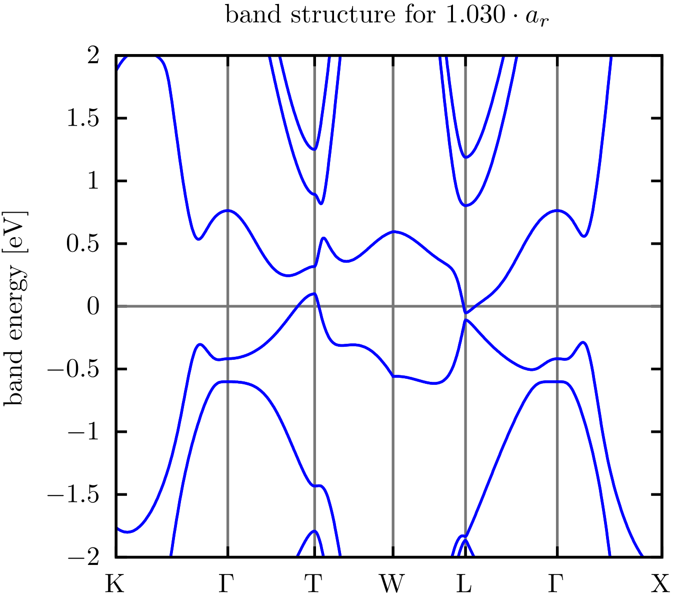

band structure for $1.030 \cdot a_r$
band energy [eV]
2
1.5
1
0.5
0
−0.5
−1
−1.5
−2
K
Γ
T
W
L
Γ
X

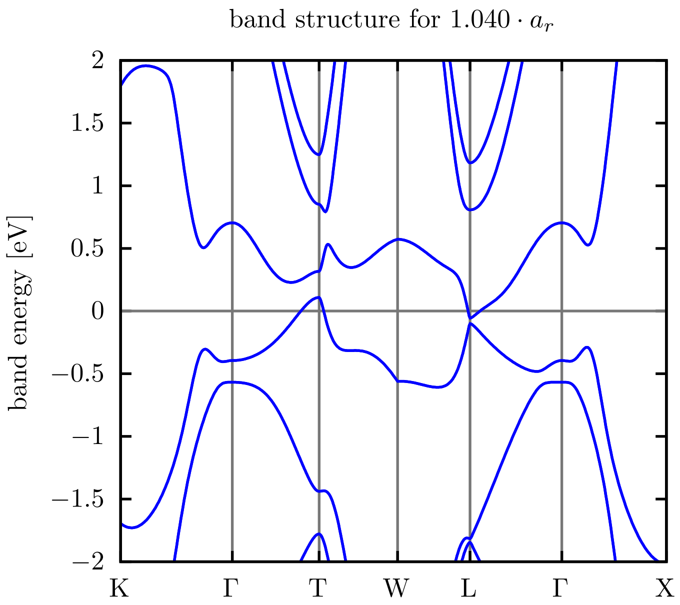
band structure for $1.040 \cdot a_r$
band energy [eV]
2
1.5
1
0.5
0
−0.5
−1
−1.5
−2
K
Γ
T
W
L
Γ
X

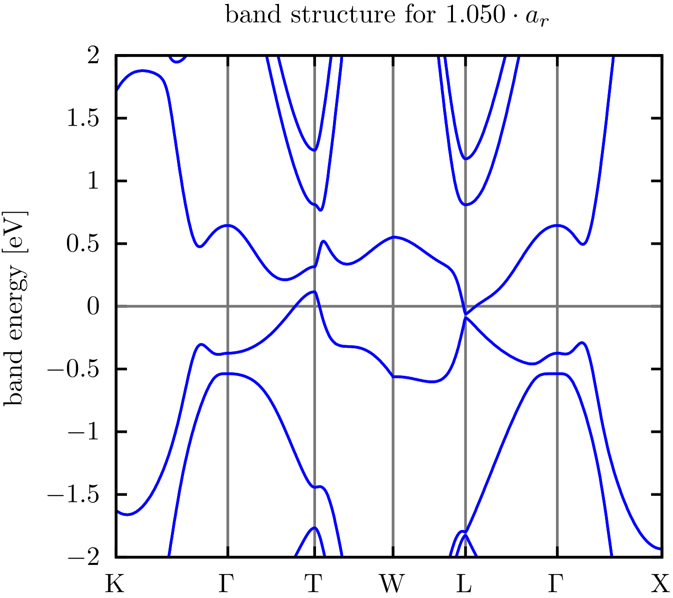

band structure for $1.050 \cdot a_r$
band energy [eV]
2
1.5
1
0.5
0
−0.5
−1
−1.5
−2
K
Γ
T
W
L
Γ
X

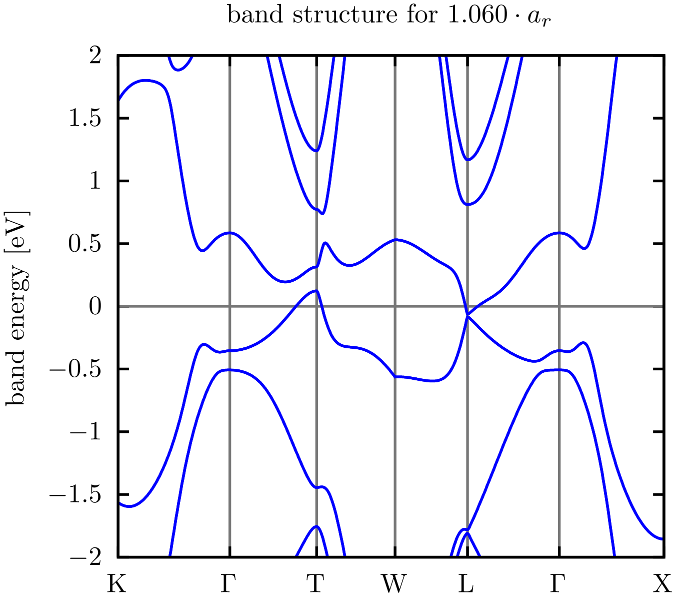

band structure for $1.060 \cdot a_r$
band energy [eV]
2
1.5
1
0.5
0
−0.5
−1
−1.5
−2
K
Γ
T
W
L
Γ
X

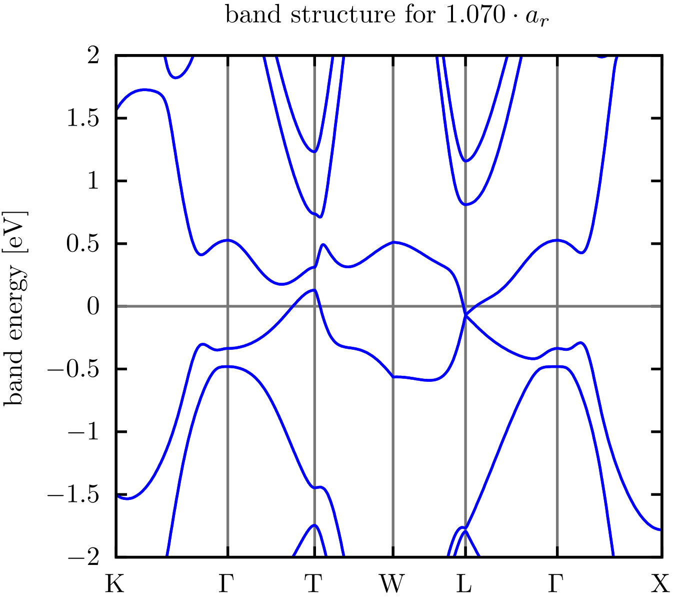

band structure for $1.070 \cdot a_r$
band energy [eV]
2
1.5
1
0.5
0
−0.5
−1
−1.5
−2
K
Γ
T
W
L
Γ
X

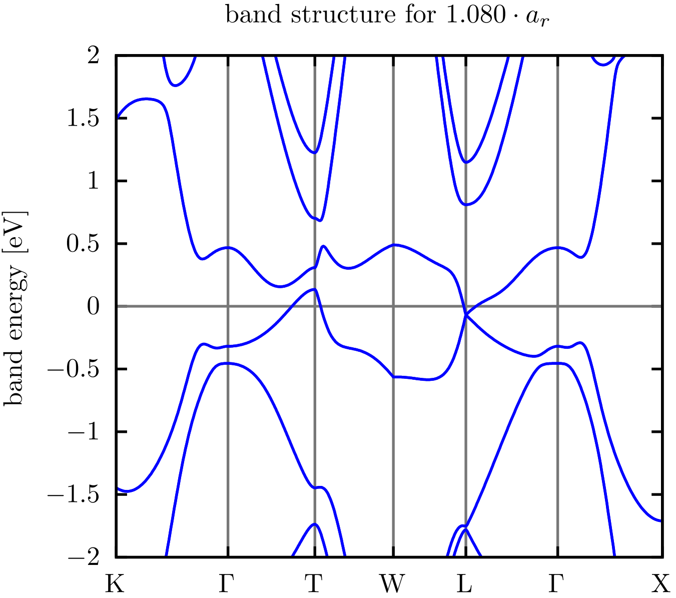

band structure for $1.080 \cdot a_r$
band energy [eV]
2
1.5
1
0.5
0
−0.5
−1
−1.5
−2
K
Γ
T
W
L
Γ
X

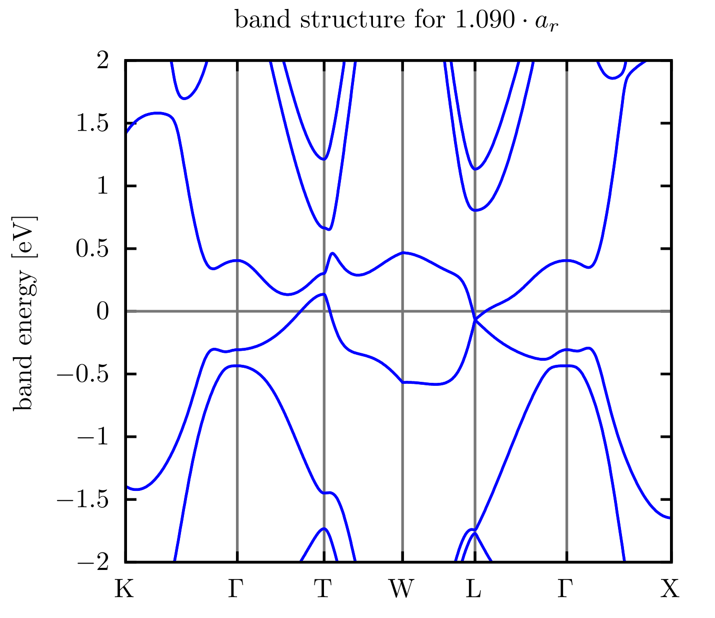
band structure for $1.090 \cdot a_r$
band energy [eV]
2
1.5
1
0.5
0
−0.5
−1
−1.5
−2
K
Γ
T
W
L
Γ
X

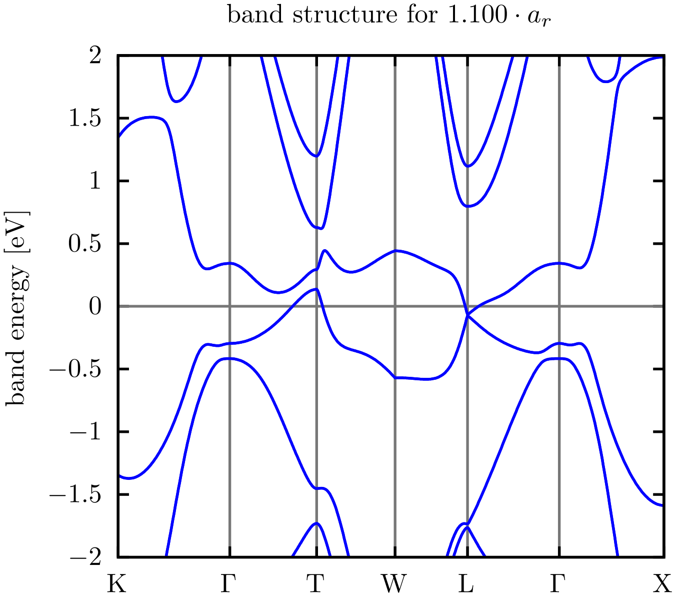

band structure for $1.100 \cdot a_r$
band energy [eV]
2
1.5
1
0.5
0
−0.5
−1
−1.5
−2
K
Γ
T
W
L
Γ
X

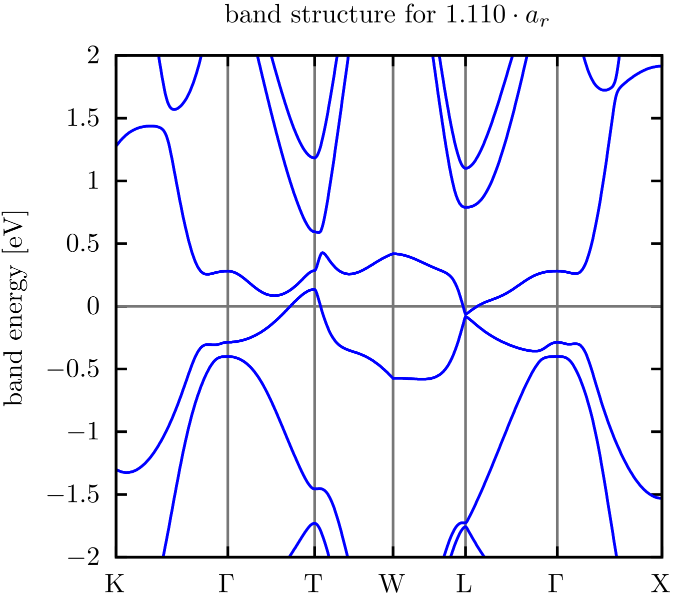

band structure for $1.110 \cdot a_r$
band energy [eV]
2
1.5
1
0.5
0
−0.5
−1
−1.5
−2
K
Γ
T
W
L
Γ
X

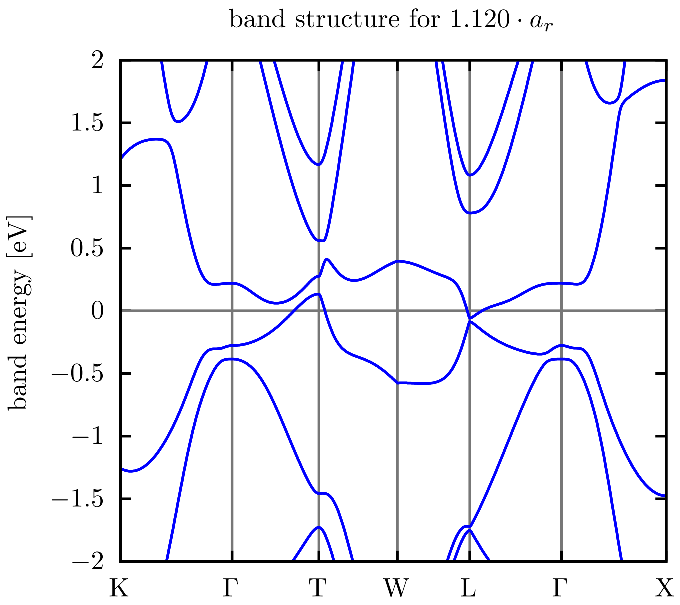

band structure for $1.120 \cdot a_r$
band energy [eV]
2
1.5
1
0.5
0
−0.5
−1
−1.5
−2
K
Γ
T
W
L
Γ
X

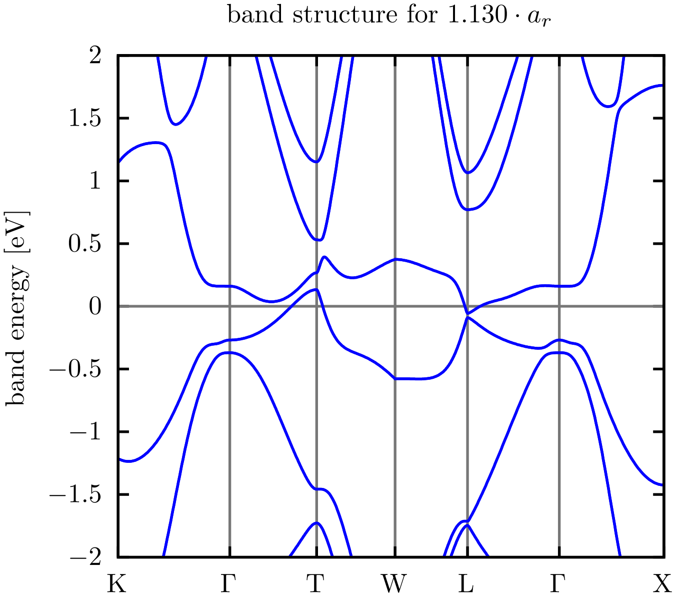
band structure for $1.130 \cdot a_r$
band energy [eV]
2
1.5
1
0.5
0
−0.5
−1
−1.5
−2
K
Γ
T
W
L
Γ
X

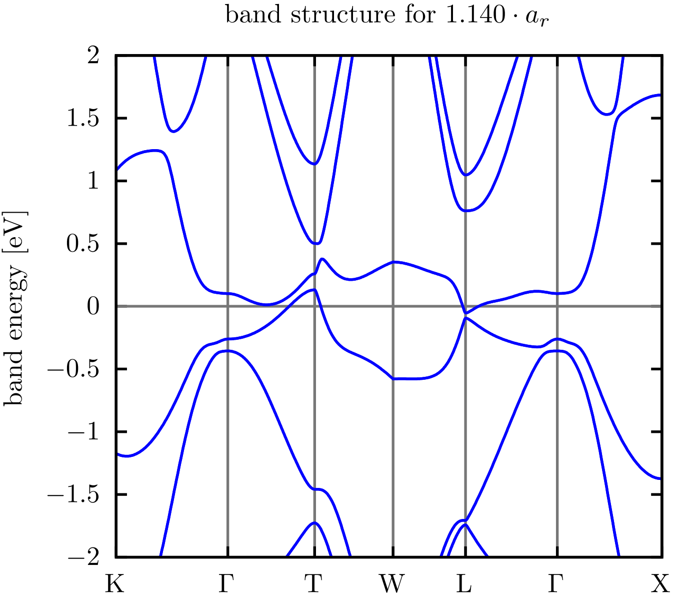

band structure for $1.140 \cdot a_r$
band energy [eV]
2
1.5
1
0.5
0
−0.5
−1
−1.5
−2
K
Γ
T
W
L
Γ
X

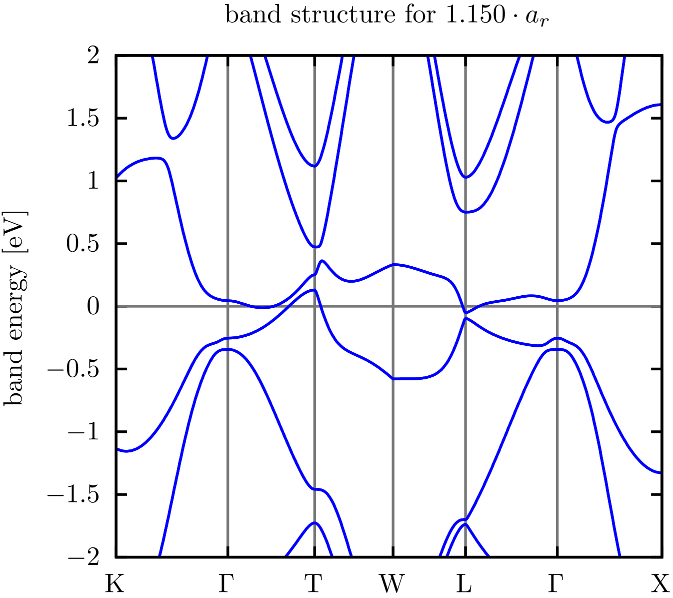

band structure for $1.150 \cdot a_r$
band energy [eV]
2
1.5
1
0.5
0
−0.5
−1
−1.5
−2
K
Γ
T
W
L
Γ
X

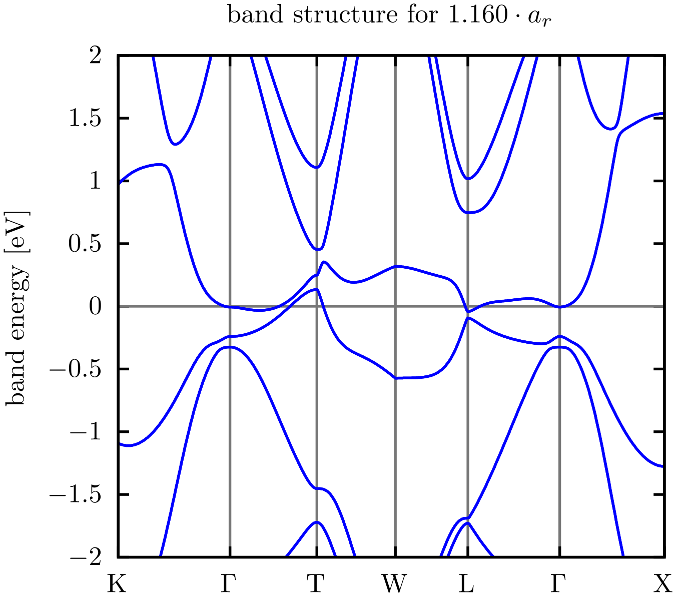

band structure for $1.160 \cdot a_r$
band energy [eV]
2
1.5
1
0.5
0
−0.5
−1
−1.5
−2
K
Γ
T
W
L
Γ
X

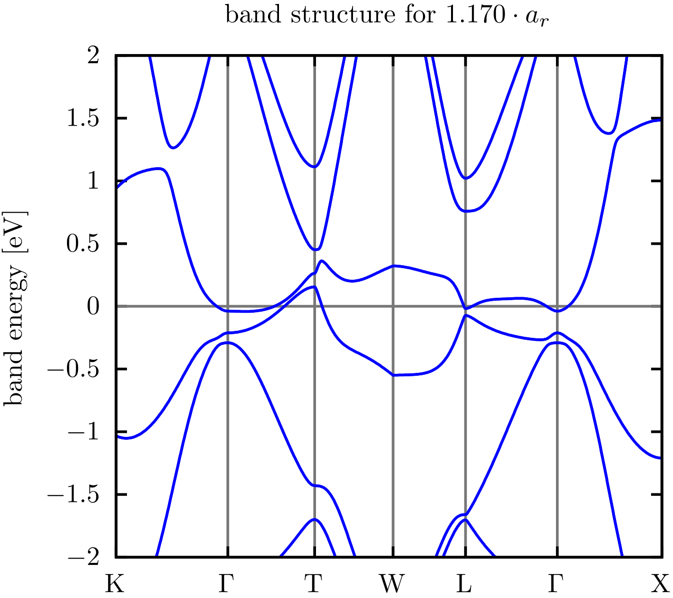

band structure for $1.170 \cdot a_r$
band energy [eV]
2
1.5
1
0.5
0
−0.5
−1
−1.5
−2
K
Γ
T
W
L
Γ
X

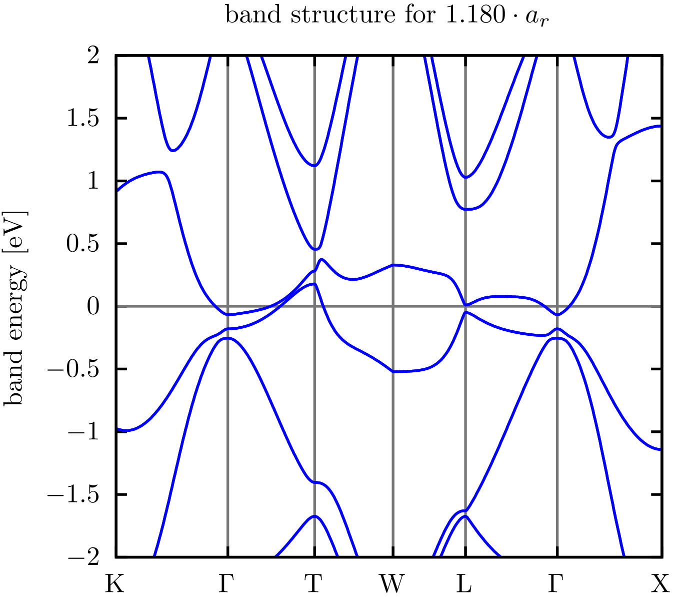

band structure for $1.180 \cdot a_r$
band energy [eV]
2
1.5
1
0.5
0
−0.5
−1
−1.5
−2
K
Γ
T
W
L
Γ
X

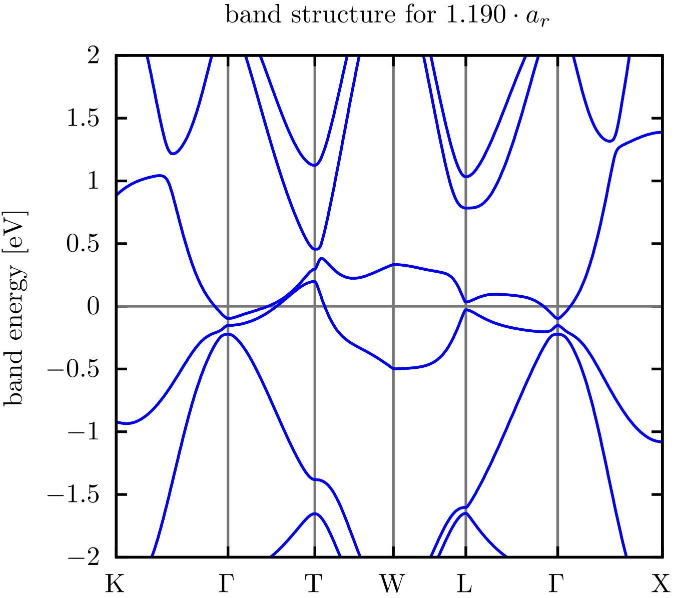
band structure for $1.190 \cdot a_r$
band energy [eV]
2
1.5
1
0.5
0
−0.5
−1
−1.5
−2
K
Γ
T
W
L
Γ
X

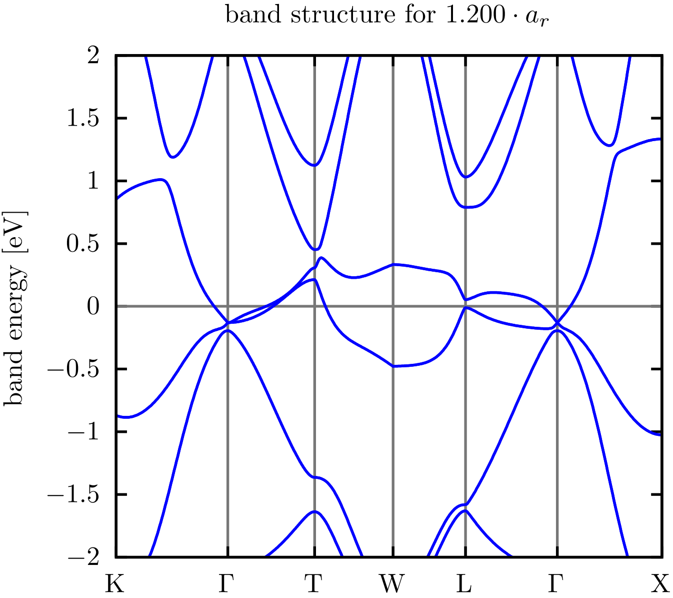
band structure for $1.200 \cdot a_r$
band energy [eV]
2
1.5
1
0.5
0
−0.5
−1
−1.5
−2
K
Γ
T
W
L
Γ
X

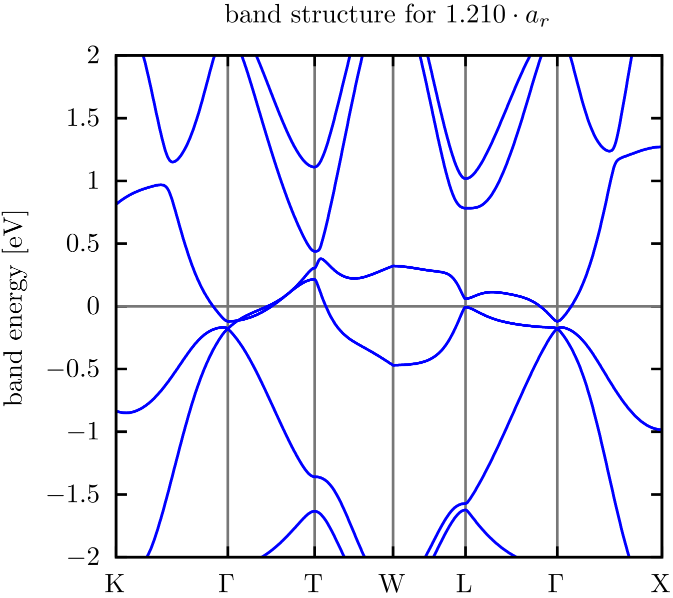
band structure for $1.210 \cdot a_r$
band energy [eV]
2
1.5
1
0.5
0
−0.5
−1
−1.5
−2
K
Γ
T
W
L
Γ
X

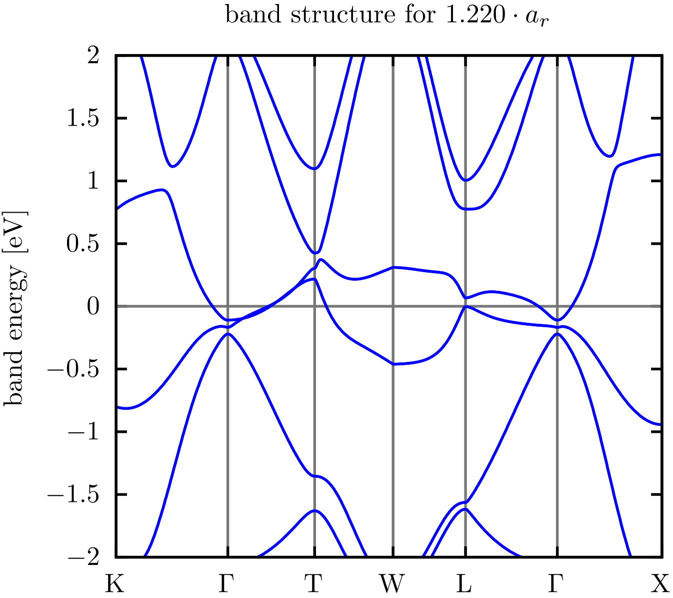

band structure for $1.220 \cdot a_r$
band energy [eV]
2
1.5
1
0.5
0
−0.5
−1
−1.5
−2
K
Γ
T
W
L
Γ
X

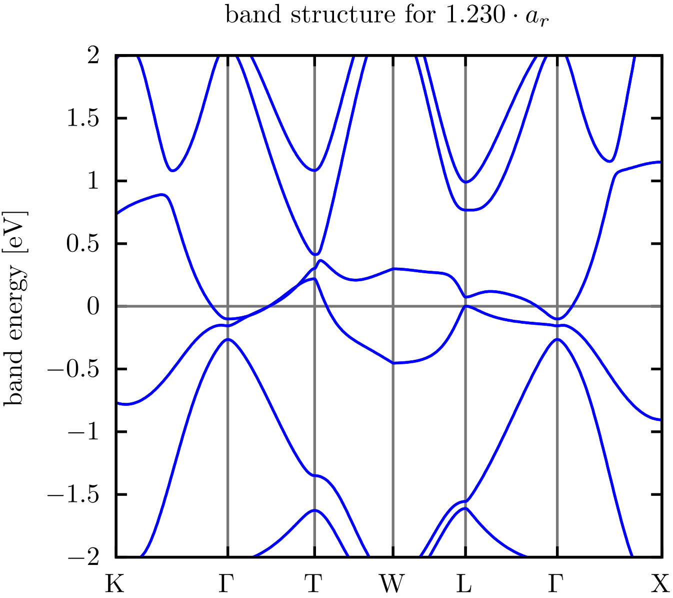
band structure for $1.230 \cdot a_r$
band energy [eV]
2
1.5
1
0.5
0
−0.5
−1
−1.5
−2
K
Γ
T
W
L
Γ
X

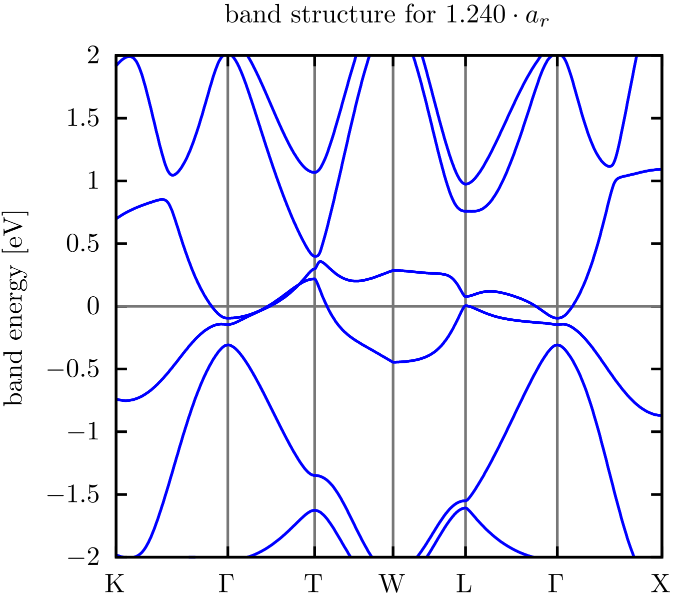
band structure for $1.240 \cdot a_r$
band energy [eV]
2
1.5
1
0.5
0
−0.5
−1
−1.5
−2
K
Γ
T
W
L
Γ
X

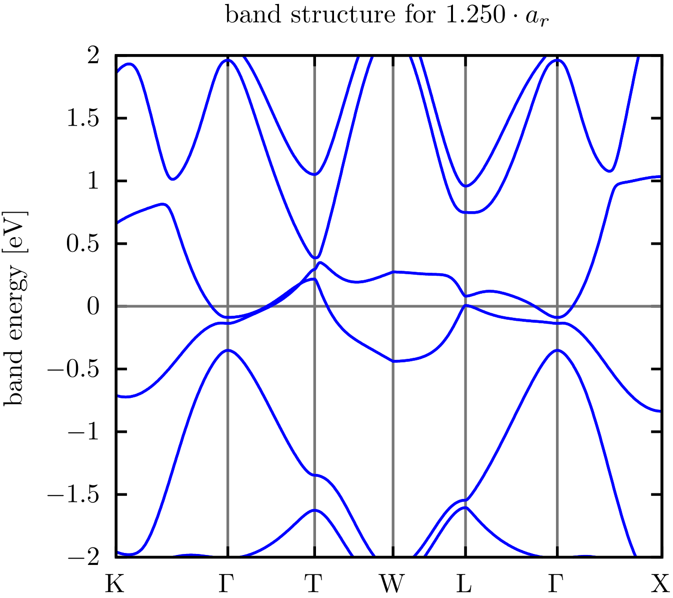

band structure for $1.250 \cdot a_r$
band energy [eV]
2
1.5
1
0.5
0
−0.5
−1
−1.5
−2
K
Γ
T
W
L
Γ
X

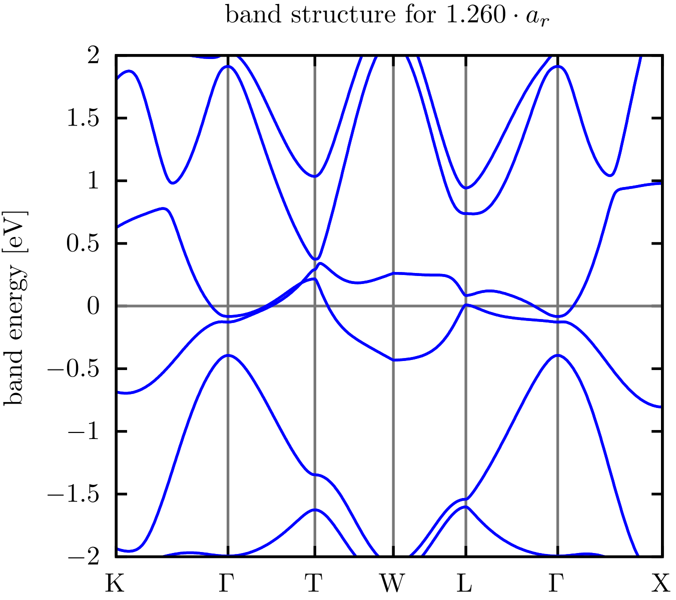

band structure for $1.260 \cdot a_r$
band energy [eV]
2
1.5
1
0.5
0
−0.5
−1
−1.5
−2
K
Γ
T
W
L
Γ
X

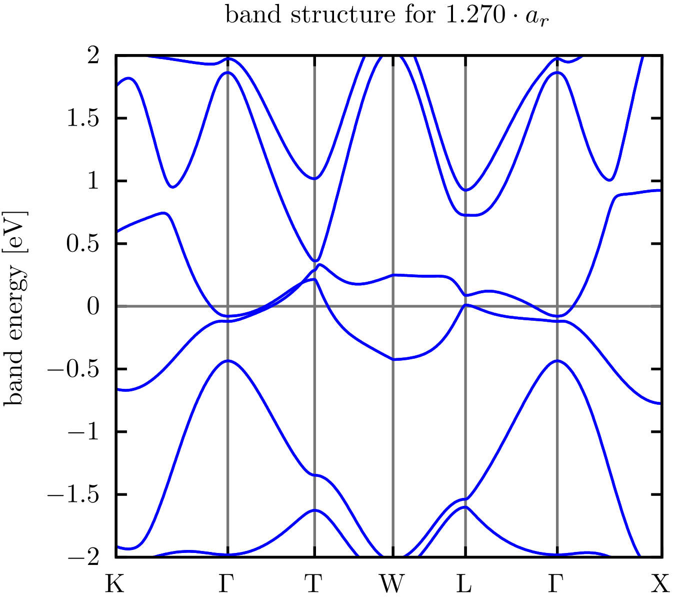

band structure for $1.270 \cdot a_r$
band energy [eV]
2
1.5
1
0.5
0
−0.5
−1
−1.5
−2
K
Γ
T
W
L
Γ
X

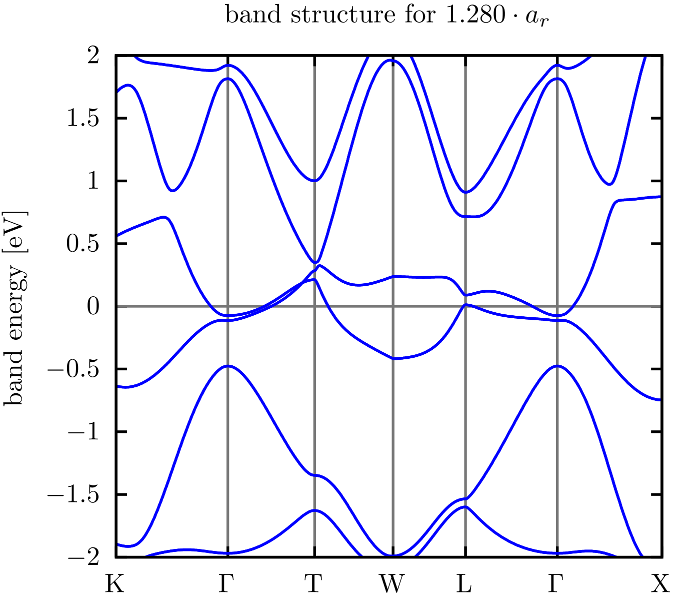

band structure for $1.280 \cdot a_r$
band energy [eV]
2
1.5
1
0.5
0
−0.5
−1
−1.5
−2
K
Γ
T
W
L
Γ
X

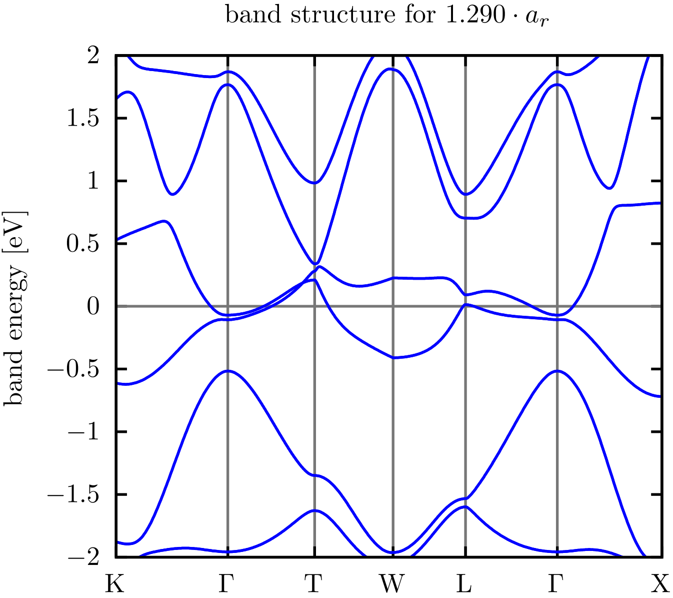

band structure for $1.290 \cdot a_r$
band energy [eV]
2
1.5
1
0.5
0
−0.5
−1
−1.5
−2
K
Γ
T
W
L
Γ
X

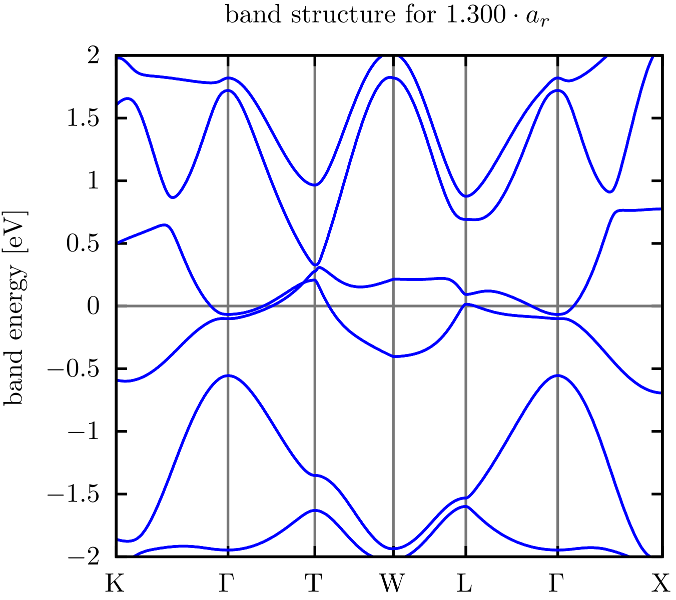
band structure for $1.300 \cdot a_r$
band energy [eV]
2
1.5
1
0.5
0
−0.5
−1
−1.5
−2
K
Γ
T
W
L
Γ
X

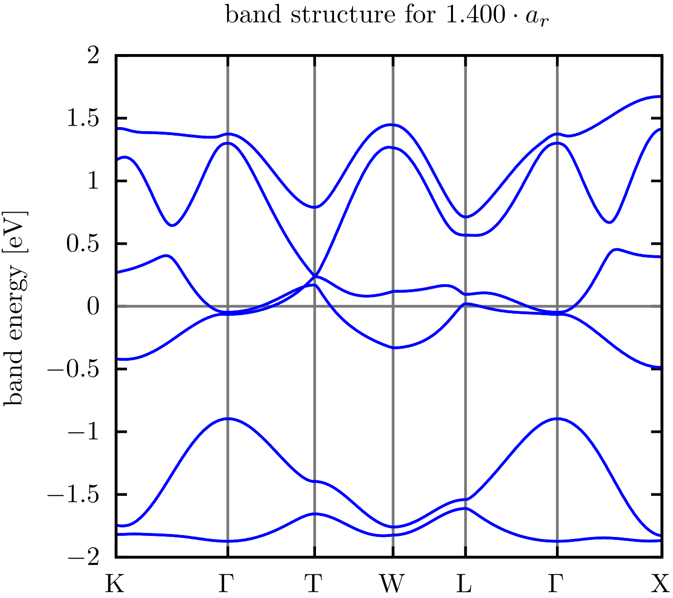
band structure for $1.400 \cdot a_r$
band energy [eV]
2
1.5
1
0.5
0
−0.5
−1
−1.5
−2
K
Γ
T
W
L
Γ
X

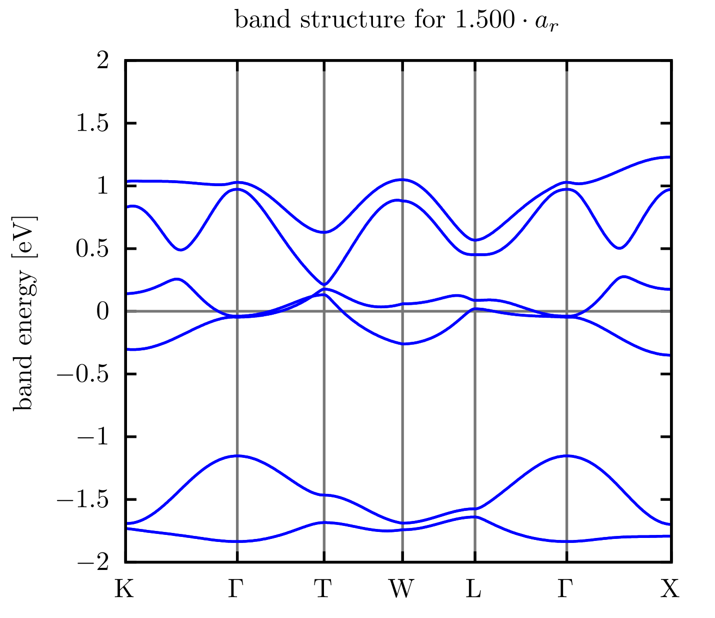
band structure for $1.500 \cdot a_r$
band energy [eV]
2
1.5
1
0.5
0
−0.5
−1
−1.5
−2
K
Γ
T
W
L
Γ
X

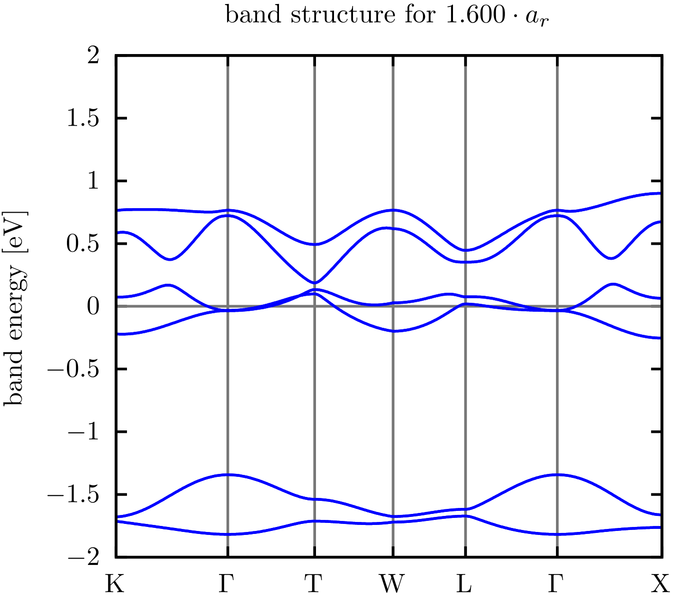

band structure for $1.600 \cdot a_r$
band energy [eV]
2
1.5
1
0.5
0
−0.5
−1
−1.5
−2
K
Γ
T
W
L
Γ
X

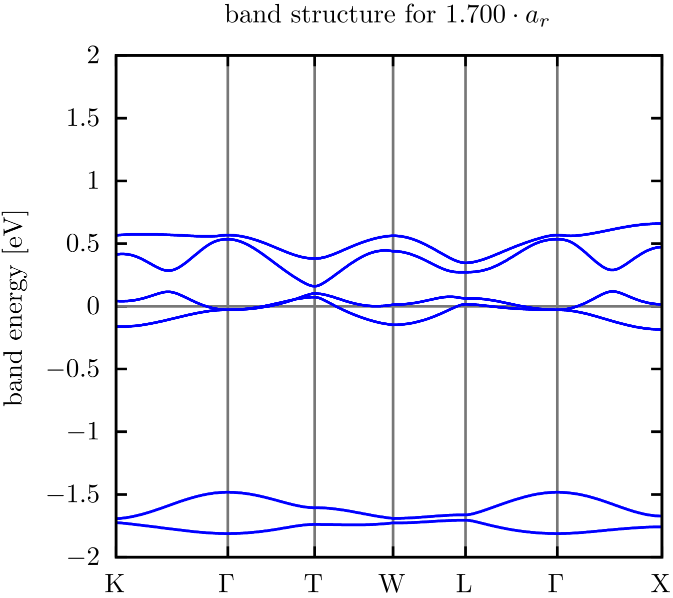

band structure for $1.700 \cdot a_r$
band energy [eV]
2
1.5
1
0.5
0
−0.5
−1
−1.5
−2
K
Γ
T
W
L
Γ
X

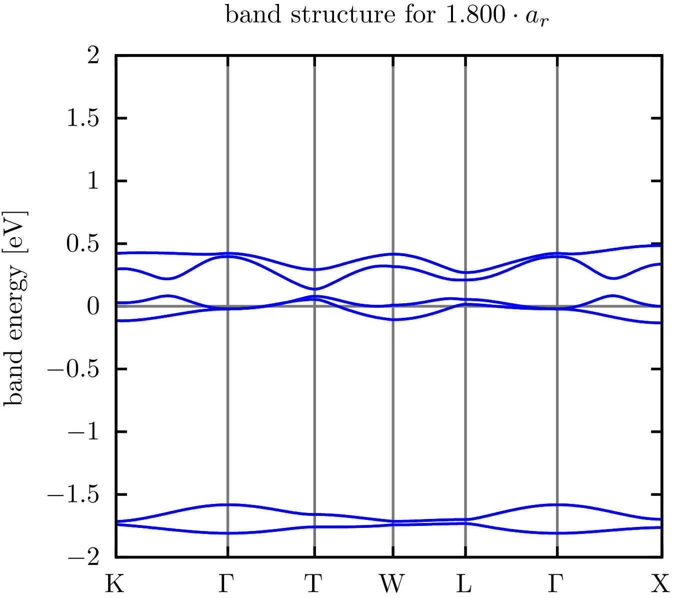

band structure for $1.800 \cdot a_r$
band energy [eV]
2
1.5
1
0.5
0
−0.5
−1
−1.5
−2
K
Γ
T
W
L
Γ
X

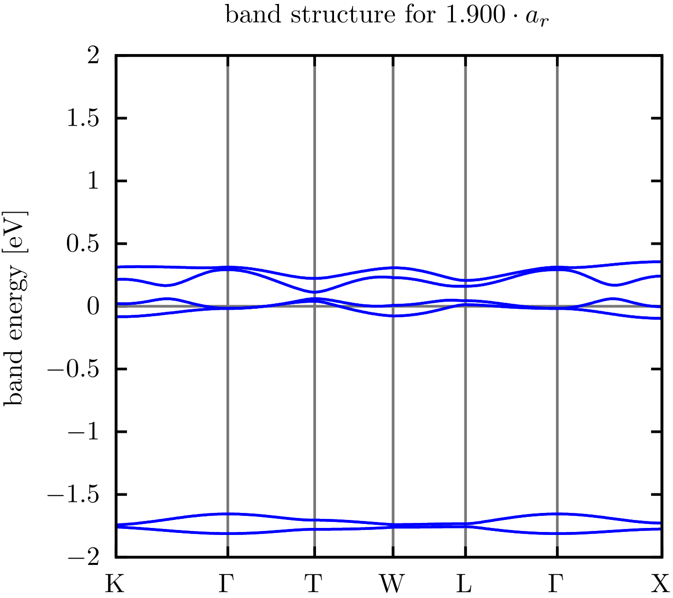

band structure for $1.900 \cdot a_r$
band energy [eV]
2
1.5
1
0.5
0
−0.5
−1
−1.5
−2
K
Γ
T
W
L
Γ
X

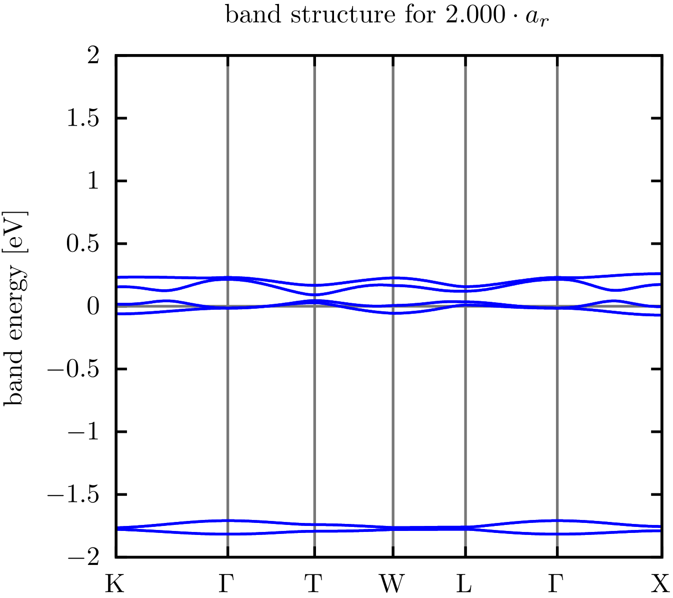
band structure for $2.000 \cdot a_r$
2
1.5
1
0.5
0
−0.5
−1
−1.5
−2
band energy [eV]
K
Γ
T
W
L
Γ
X

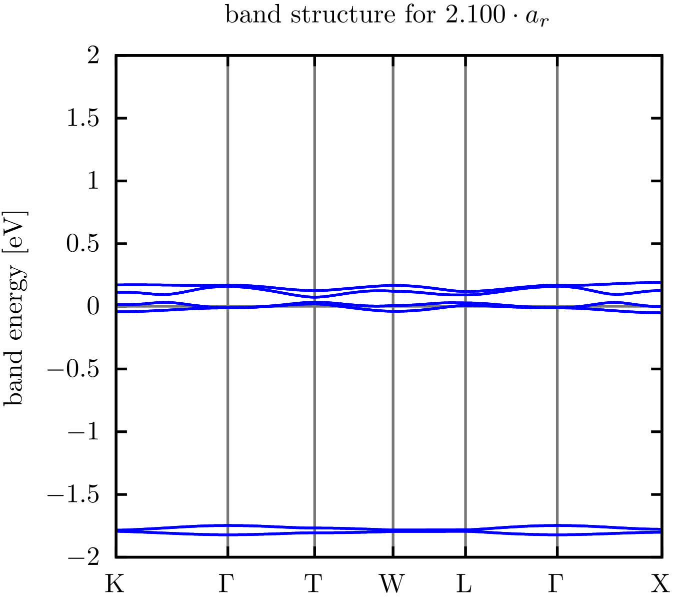

band structure for $2.100 \cdot a_r$
band energy [eV]
2
1.5
1
0.5
0
−0.5
−1
−1.5
−2
K
Γ
T
W
L
Γ
X

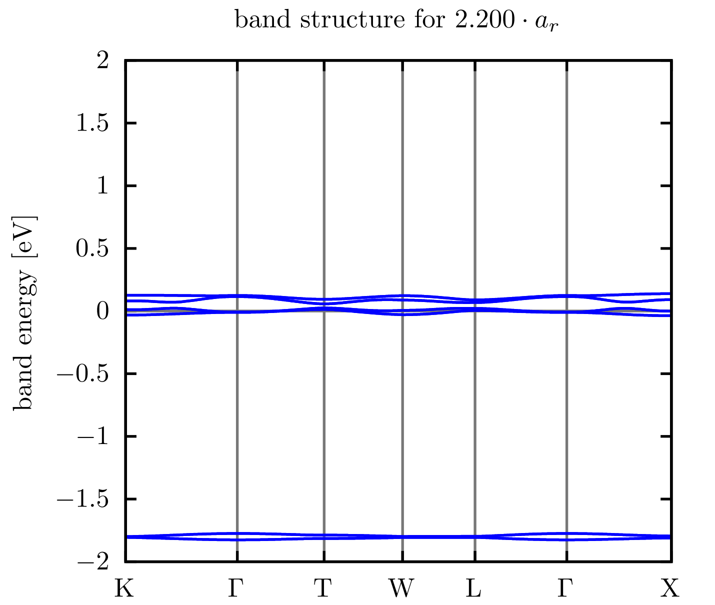

band structure for $2.200 \cdot a_r$
band energy [eV]
2
1.5
1
0.5
0
−0.5
−1
−1.5
−2
K
Γ
T
W
L
Γ
X

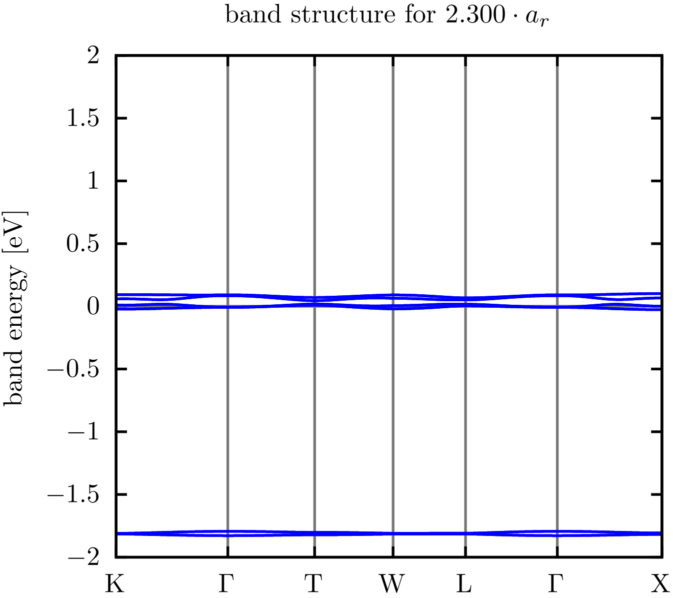
band structure for $2.300 \cdot a_r$
band energy [eV]
2
1.5
1
0.5
0
−0.5
−1
−1.5
−2
K
Γ
T
W
L
Γ
X

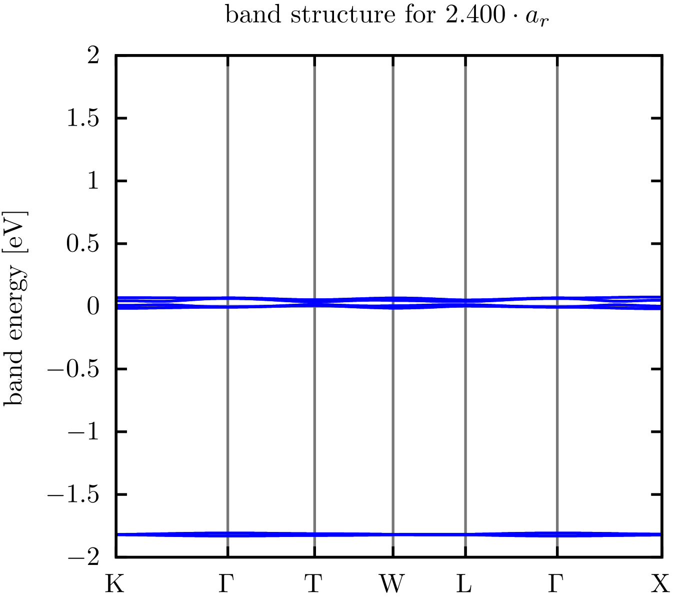
band structure for $2.400 \cdot a_r$
band energy [eV]
2
1.5
1
0.5
0
−0.5
−1
−1.5
−2
K
Γ
T
W
L
Γ
X

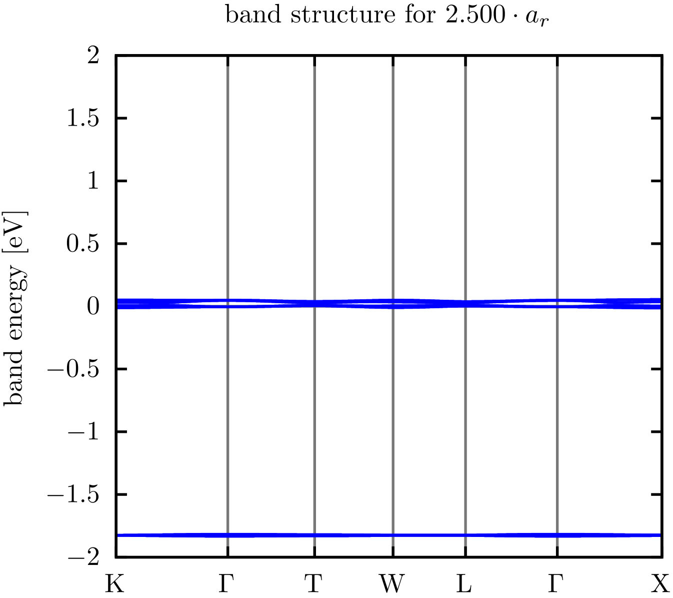
band structure for $2.500 \cdot a_r$
band energy [eV]
2
1.5
1
0.5
0
−0.5
−1
−1.5
−2
K
Γ
T
W
L
Γ
X

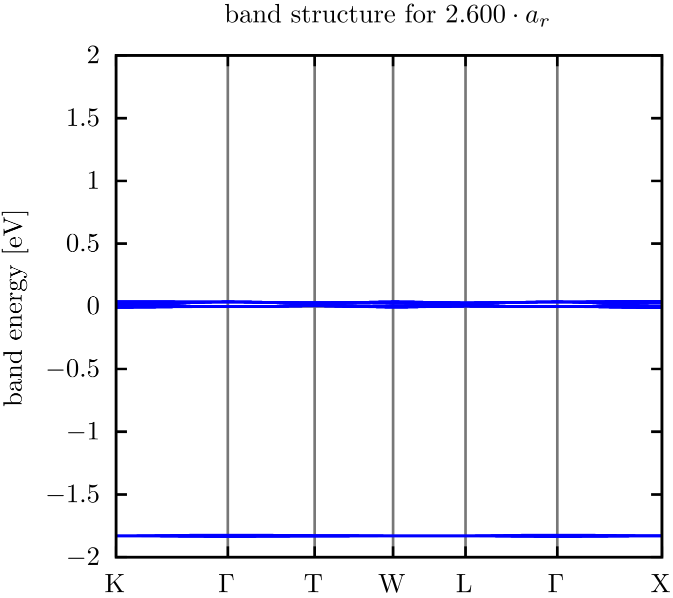
band structure for $2.600 \cdot a_r$
band energy [eV]
2
1.5
1
0.5
0
−0.5
−1
−1.5
−2
K
Γ
T
W
L
Γ
X

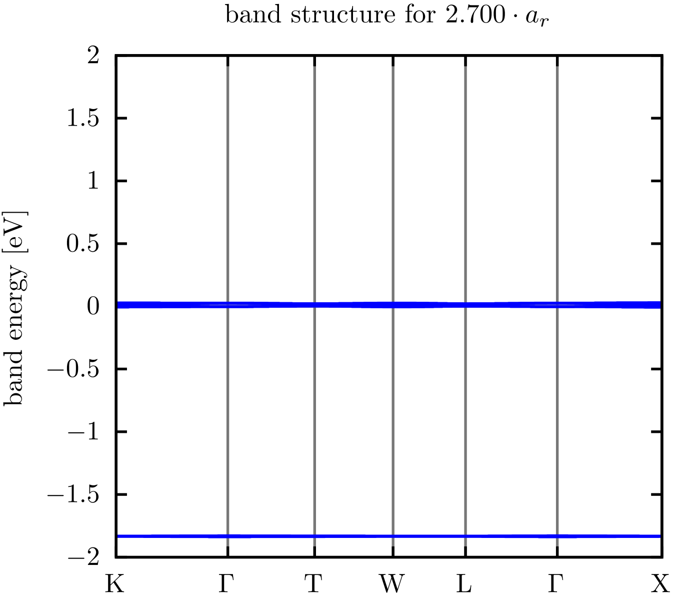

band structure for $2.700 \cdot a_r$
band energy [eV]
2
1.5
1
0.5
0
−0.5
−1
−1.5
−2
K
Γ
T
W
L
Γ
X

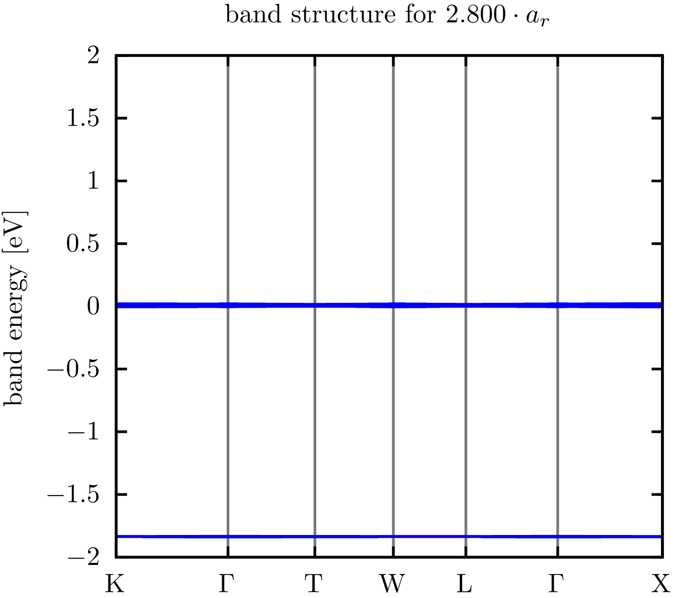

band structure for $2.800 \cdot a_r$
band energy [eV]
2
1.5
1
0.5
0
−0.5
−1
−1.5
−2
K
Γ
T
W
L
Γ
X

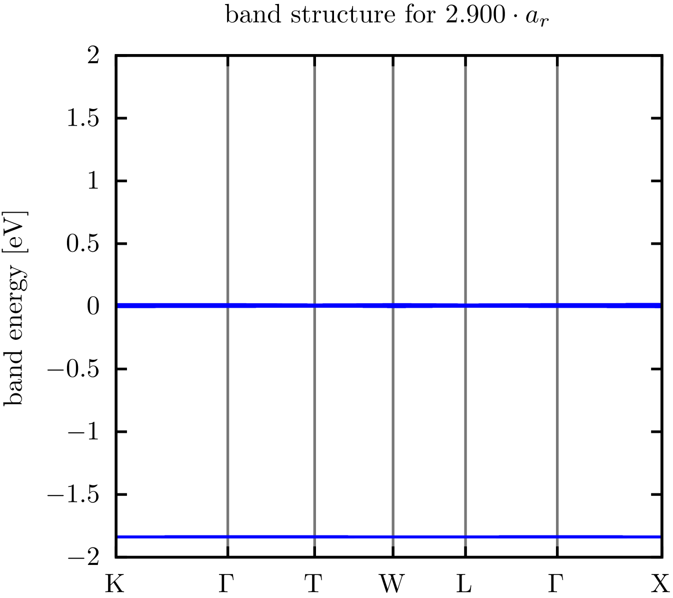

band structure for $2.900 \cdot a_r$
band energy [eV]
2
1.5
1
0.5
0
−0.5
−1
−1.5
−2
K
Γ
T
W
L
Γ
X

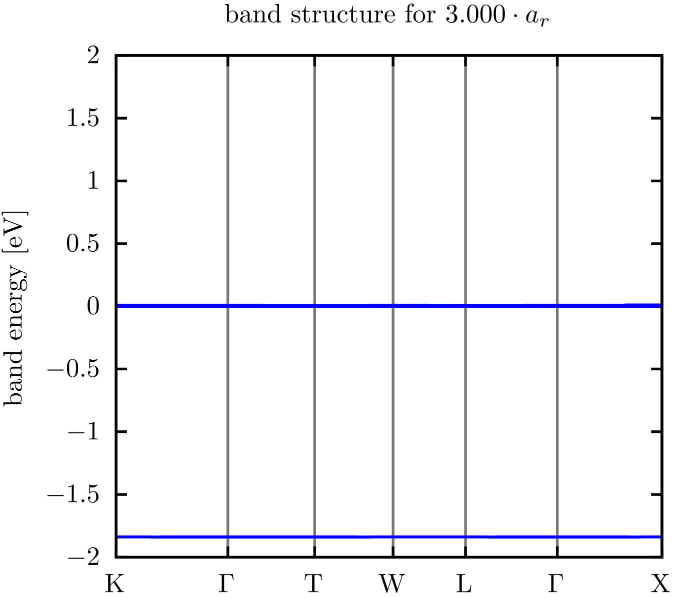

band structure for $3.000 \cdot a_r$
band energy [eV]
2
1.5
1
0.5
0
−0.5
−1
−1.5
−2
K
Γ
T
W
L
Γ
X
